# Supplementary material for: Division-of-Thoughts: Harnessing Hybrid Language Model Synergy for Efficient On-Device Agents
Source: arXiv:2502.04392 source file (2025-02-06)
Supplement: Supplementary file 1 [file Appendix1.tex]

\section{Appendix 1}

\subsection{Part One}

Part 1.1

\subsection{Part Two}

Part 1.2
