# Supplementary material for: Division-of-Thoughts: Harnessing Hybrid Language Model Synergy for Efficient On-Device Agents
Source: arXiv:2502.04392 source file (2025-02-06)
Supplement: Supplementary file 2 [file Appendix2.tex]

\section{Appendix 2}

Part 2
